# Supplementary material for: Spontaneous Segregation of Self-Propelled Particles with Different Motilities
Source: arXiv:1110.2479 ancillary file (2011-10-13)
Supplement: Supplementary file 1 [file SupplementalInformation.pdf]

# Spontaneous Segregation of Self-Propelled Particles with Different Motilities: Supplemental Information

Samuel R. McCandlish, Aparna Baskaran, and Michael F. Hagan
*Martin A. Fisher School of Physics, Brandeis University, Waltham, MA, 02454*
(Dated: October 13, 2011)

In this supplemental material, we first provide further information about the clustering behavior of the rods, including cluster size distributions and our method for identifying clusters. We also explain the relationship between the segregation parameter $\hat{\sigma}$ and the mean cluster size discussed in the main text. Then we present snapshots from simulations of various parameters to display the behavior of the mixed system as a function of motile fraction. Finally, we present various pair correlation functions that illustrate the anatomies of clusters and can be measured in experiments [1].

*1. Clustering and swarming:* Various representative cluster size distributions are shown in Fig. S1. Due to a lack of statistics at large cluster sizes, the cluster size distributions are shown averaged over bins of width 0.1 in $\log n$. For low $\phi$, $L$, $f_{\rm a}$, and Pe, the distributions follow a power law with an exponential cutoff. Increasing $\phi$, $L$, $f_{\rm a}$, and Pe yields distributions that 'pile up' at large cluster sizes, with the most extreme example ($L = 21$, $\phi = 0.8$, Pe $= 120$) exhibiting system-sized clusters. The forms of these cluster size distributions are qualitatively similar to those observed by [2]. We find that segregation occurs even for parameters well below the threshold at which this plateau develops in the cluster size distribution.

*2. Determination of the Segregation Order Parameter:* The method for determining the segregation parameter $\sigma_{\rm a}(b)$ as described in the main text is shown in Fig. S2 as a function of the discretization box size $b$. In order to account for the nonzero value of $\sigma_a(b)$ at zero Péclet number, we subtract the same function $\sigma_0(b)$, computed for a system with the same parameter values except Pe $=$ 0. This function is a nonmonotonic function of the box size $b$. Then, we define the segregation order parameter $\hat{\sigma}$ to be the maximum value of $\sigma_{\rm a}(b) - \sigma_0(b)$ over all $b$.

*3. Snapshots from Simulations:* We display in Figs. S3,S4,S5,S6 snapshots from simulations at various parameters. In these snapshots, active rods are colored red, and passive rods are colored blue. Figures S4,S5,S6 are arranged identically to figures 3(b-d) in the main text to facilitate comparison with the segregation order parameter $\hat{\sigma}$. Figure S3 displays the segregation behavior at high area fraction. These snapshots display the variety of emergent behavior that occurs at various system parameters.

At low motile fraction $f_{\rm a}$, we find active clusters in a passive "gas", and the simple dependence of segregation on the cluster size distribution is clear. At higher $f_{\rm a}$, the passive rods form "herds" which also increase the degree of segregation. At high $f_{\rm a}$ and high area fraction $\phi$ (Fig. S3), the "herds" of passive rods are most evident.

*4. Relationship Between Clustering and Segregation:* The enhanced local alignment due to rod propulsion gives rise to collective motion of polar clusters. We define a cluster as in [1, 2]. Two active rods are considered to be in the same cluster if their representative line segments are within $3\sigma$ of each other, and their relative angle is less than $\pi/6$. Traversing these connections yields a set of clusters. A single unconnected rod is counted as a cluster of size one. We do not consider passive rods when identifying clusters in this way.

To measure the degree of segregation within clusters, we also implemented an alternative algorithm that identifies clusters in a manner independent of rod species. In this algorithm, two rods are connected if their average relative velocity over a time $\tau$ is smaller than a threshold value $v_{\rm max}$. The size of clusters chosen by this method was sensitive to the parameters $\tau$ and $v_{\rm max}$, but the calculation confirmed that clusters with a motile fraction between 0.2 and 0.8 are rare. Typically clusters contain at least 99% active rods.

As noted in the main text, there is a close relationship between the mean cluster size $\langle n_{\rm C} \rangle$ and the segregation parameter $\hat{\sigma}$. This relationship holds under conditions for which clusters are nearly pure and there is a one-to-one mapping between the mean cluster size and the cluster size distribution. Under these conditions, rods well within the interior of a cluster are almost entirely surrounded by other rods of the same species and are thus segregated, while rods at cluster interfaces have a mixture of neighbors and thus tend to be integrated. Therefore, the segregation parameter can be estimated by calculating the fraction of rods $f_{\rm int}$ which are found in the interiors of clusters.

To estimate $f_{\rm int}$ we represent a cluster of size $n_{\rm C}$ as a rectangle of width $w$ and length $2w$, which consists entirely of of active rods with number density $L^{-1}$, so that $w = \sqrt{n_{\rm C} L/2}$. This approximation is based on the typical aspect ratio of clusters and the fact that clusters are close to 99% pure for conditions where the relationship holds. The value of $w$ is obtained from the distribution of cluster sizes for a given parameter set. The area of the interior of a cluster $A_{\rm int}$ is defined as the area of the region that lies a distance of at least $b/2$ from the edge of the rectangle, where $b$ is the box side length used to calculate the segregation parameter. If $w < b$ then there is no interior, $A_{\rm int} = 0$, and otherwise $A_{\rm int} = (w - b)(2w - b)$. Then, the *interior fraction* at a given set of parameters is defined from the cluster size distribution $\Pi(n)$ for that parameter set as the total interior of all clusters divided

by the total area of all clusters:

$$f_{\mathrm{int}} = \frac{\sum_{n=1}^{\infty} \Pi(n) A_{\mathrm{int}}}{\sum_{n=1}^{\infty} \Pi(n) A}.$$

As shown in Fig. S7, comparing this parameter with the segregation parameter shows a strong correlation, which corresponds to the correlation between the mean cluster size and segregation parameter presented in the main text.

*5. Pair Correlation Functions:* We compute pair correlation functions $G(x,y)$ between the different rod species as follows. For a given rod $i$, we define a local coordinate system according to the reference frame of rod $i$, with $\hat{x}_i$ as the unit vector in the direction perpendicular to the axis of rod $i$ and $\hat{y}_i$ as the unit vector parallel to the rod's axis. Then, the two dimensional pair interspecies correlation function is defined as

$$G_{\mathrm{XY}}(x,y) = \frac{1}{\rho} \left\langle \sum_{j \neq i} \delta[x\hat{x}_i + y\hat{y}_i - (\vec{r}_i - \vec{r}_j)] \right\rangle_i$$

where the average is taken only over rods $i$ of species X, and the sum is only over rods $j$ of species Y, and the species can be either P (passive) or A (active). Similarly, the polar and nematic orientation correlation functions are defined by

$$C_{\mathrm{P,XY}}(x,y) = \langle (\hat{y}_i \cdot \hat{y}_j) \delta[x\hat{x}_i + y\hat{y}_i - (\vec{r}_i - \vec{r}_j)] \rangle_{ij}$$

and

$$C_{\mathrm{N,XY}}(x,y) = \left\langle (2(\hat{y}_i \cdot \hat{y}_j)^2 - 1) \delta[x\hat{x}_i + y\hat{y}_i - (\vec{r}_i - \vec{r}_j)] \right\rangle_{ij}$$

These pair correlation functions are shown in Figs. S8, S9, S10 for parameters $L = 21$, $\phi = 0.2$, Pe= 120.The correlation functions $G_{\mathrm{AA}}$ and $G_{\mathrm{PP}}$ indicate the clustering of active and passive rods, and show the approximate shape and size of the clusters. Also, the region less than 1 near the origin of $G_{\mathrm{AP}}$ and $G_{\mathrm{PA}}$ indicates a deficiency in the density of passive rods near active ones and vice verse, which is a consequence of segregation. The empty regions behind active clusters which are devoid of passive rods are seen clearly in $G_{\mathrm{AP}}(x,y)$ as a deficiency at $y < 0$. As a consequence, passive rods behind active clusters are aligned in the same direction as the cluster, as seen in $C_{\mathrm{N,AP}}$. The regions of aligned rods in $C_{\mathrm{N,PA}}$ are due to the effect of clusters colliding with passive rods, pushing them into ordered regions.

[1] H. P. Zhang, A. Be'er, E.-L. Florin, and H. L. Swinney, Proc. Natl. Acad. Sci. U. S. A. **107**, 13626 (2010).

[2] Y. Yang, V. Marceau, and G. Gompper, Phys. Rev. E **82**, 1 (2010).

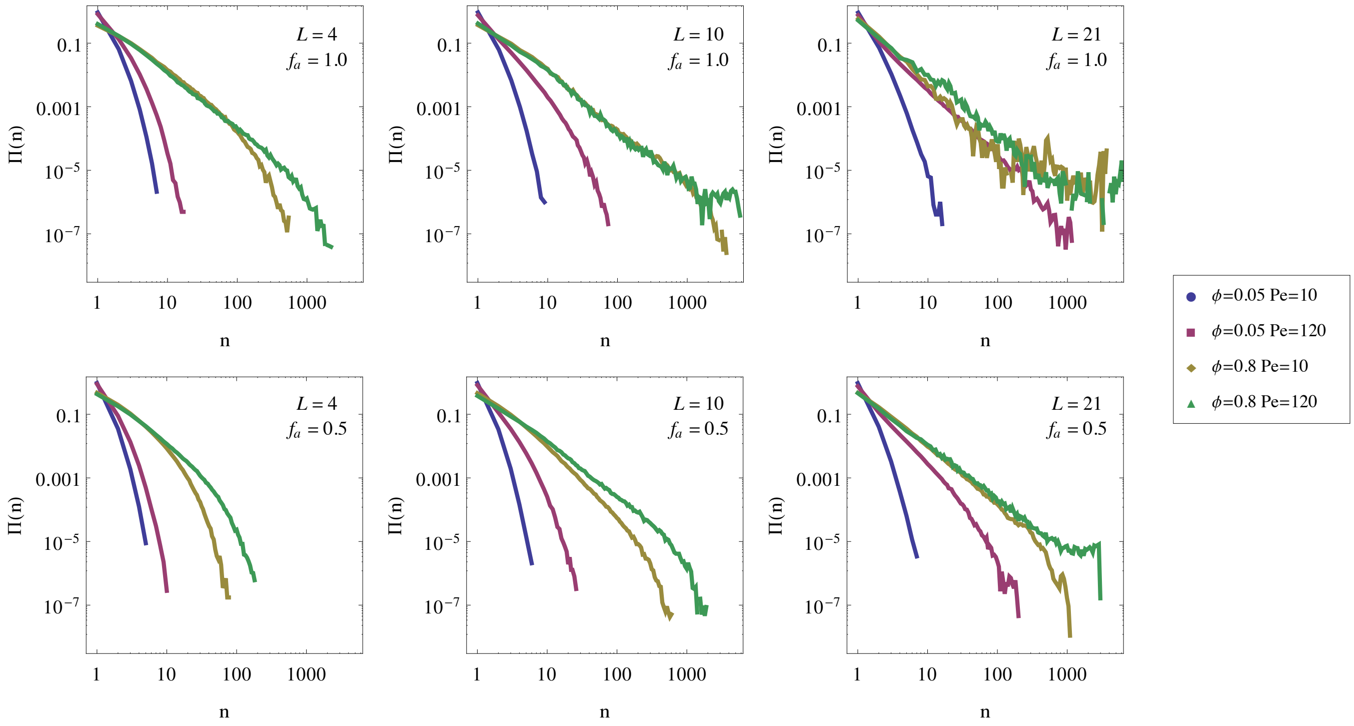


Figure S1. Cluster size distributions $\Pi(n)$ compared across aspect ratio $L$, motile fraction $f_a$, area fraction $\phi$, and Péclet number Pe. The top row corresponds to pure systems ($f_a = 1$) and the bottom row corresponds to mixed systems ($f_a = 0.5$).

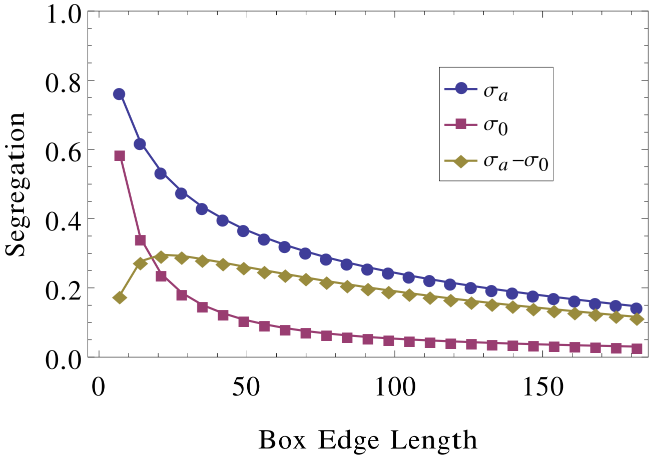


Figure S2. Determination of the segregation parameter $\hat{\sigma}$ for $L = 10, \phi = 0.2, \mathrm{Pe} = 120$. The parameters are calculated for varying box sizes in the mixed case ($\sigma_a$) and the zero force case ($\sigma_0$). The segregation parameter $\hat{\sigma}$ is defined as the maximum difference between $\sigma_a$ and $\sigma_0$.

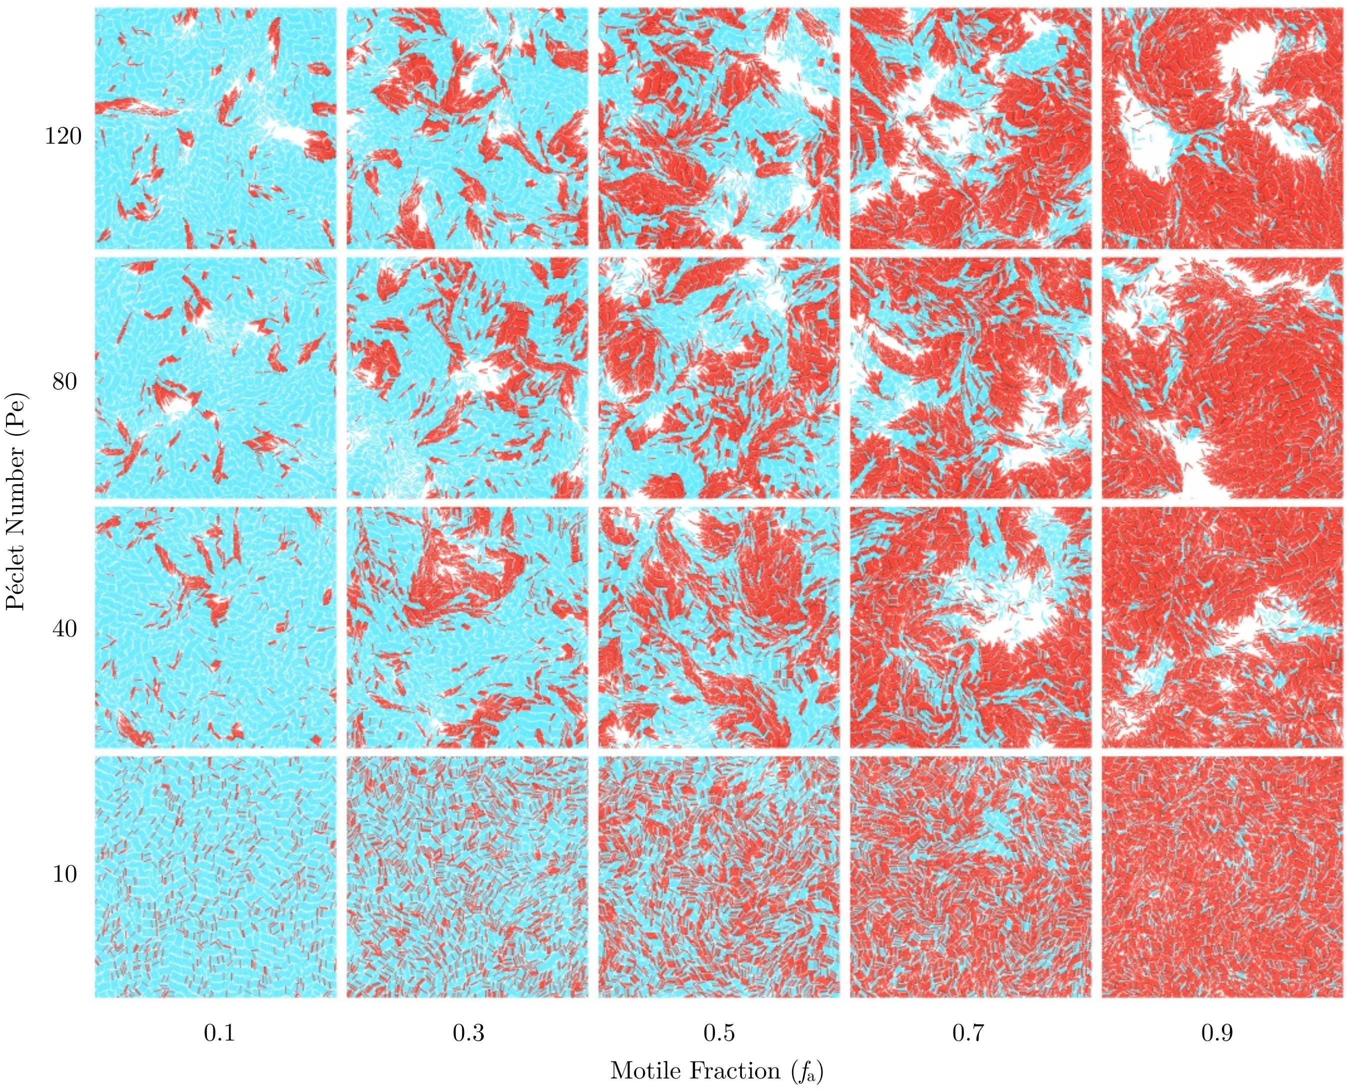


Figure S3. Snapshots from simulations of varying Pe, $f_a$ with fixed $L = 10$, $\phi = 0.8$.

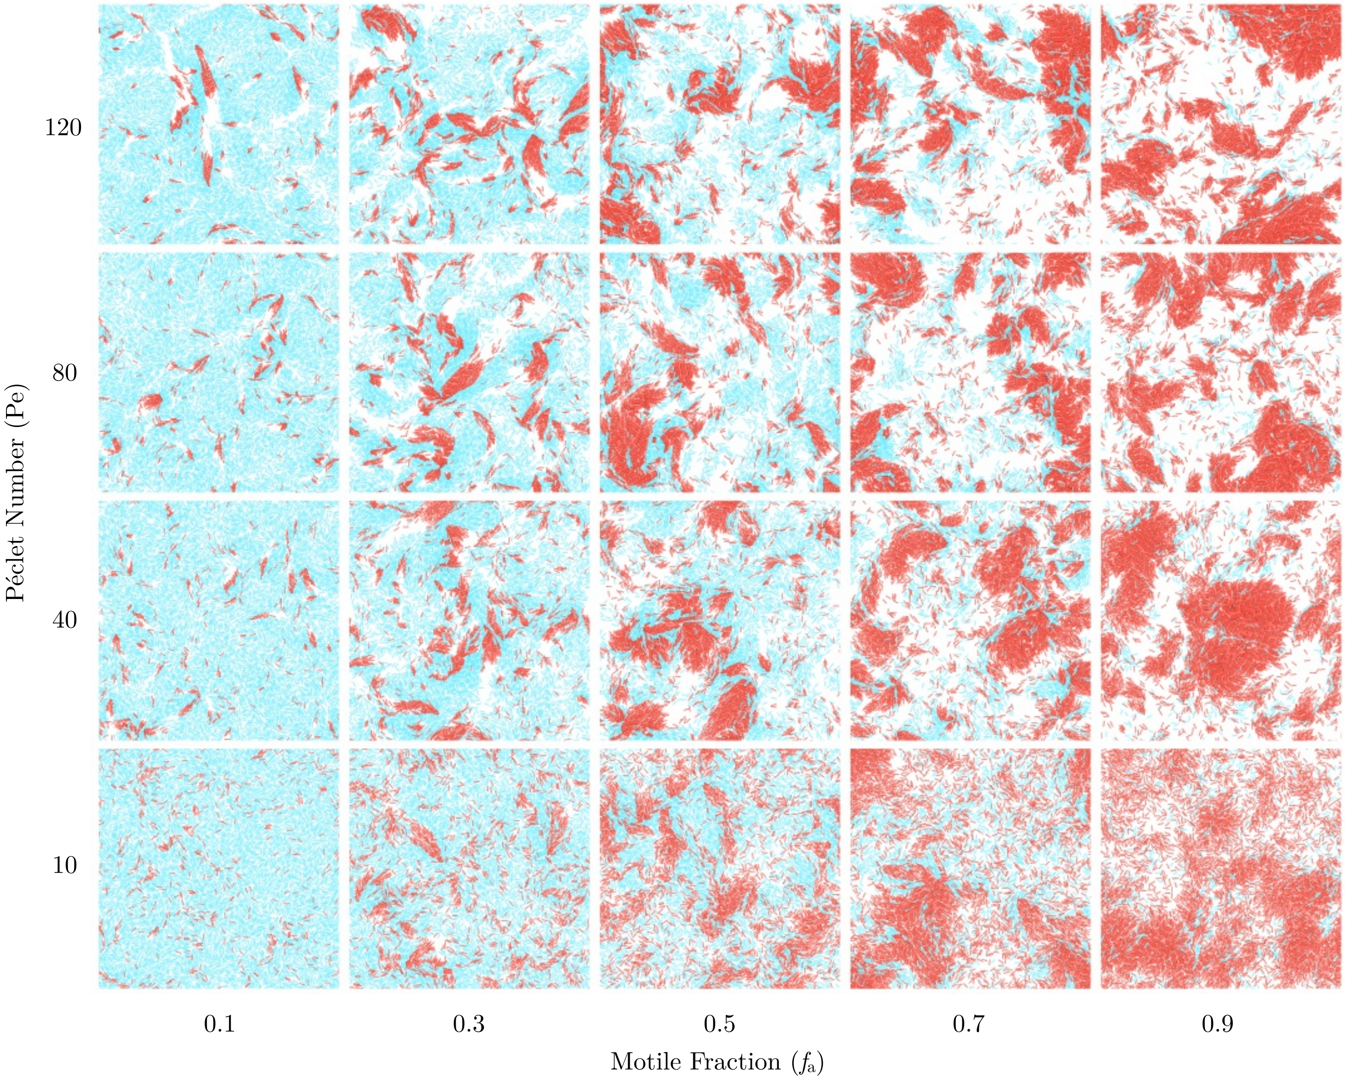


Figure S4. Snapshots from simulations of varying Pe, $f_{\mathrm{a}}$ with fixed $L = 10$, $\phi = 0.4$.

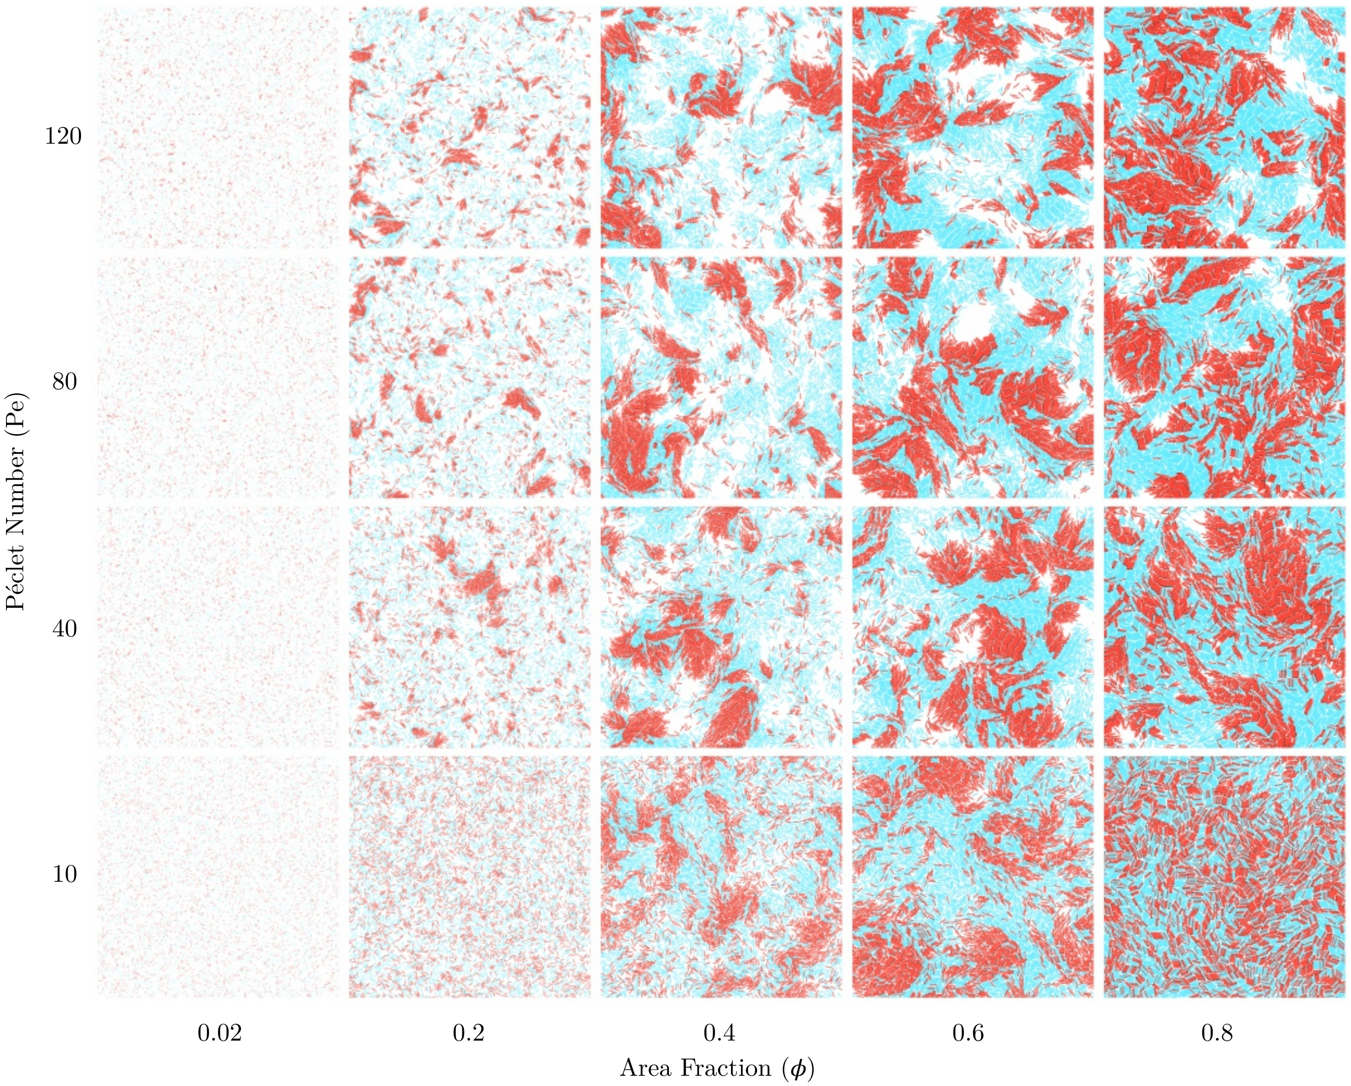


Figure S5. Snapshots from simulations of varying Pe, $\phi$ with fixed $L = 10$, $f_{\mathrm{a}} = 0.5$.

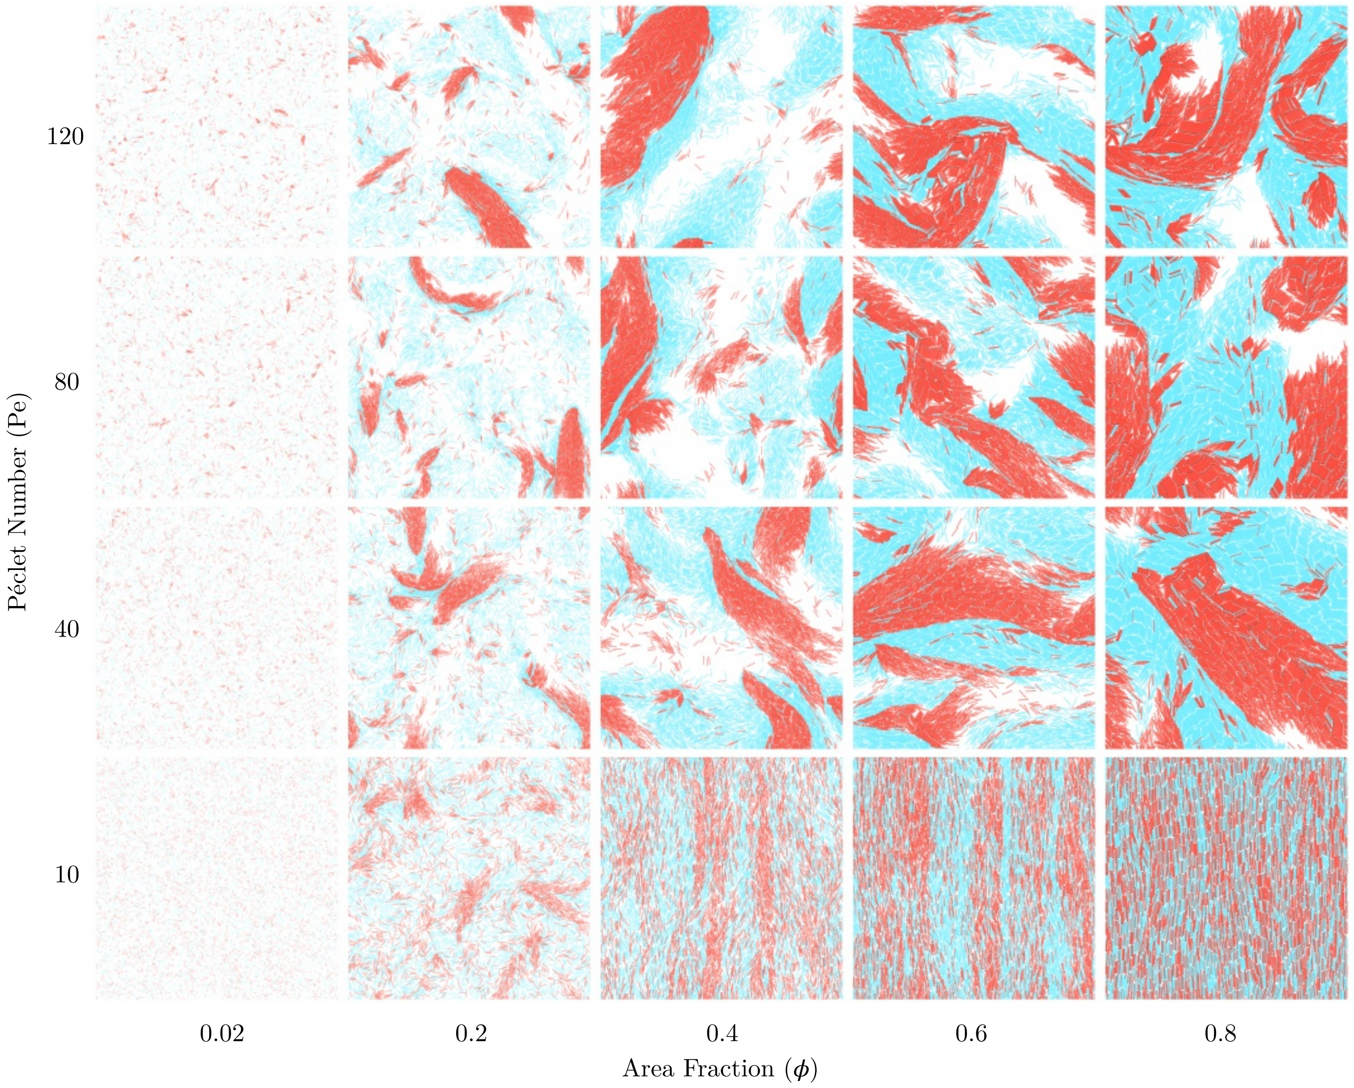


Figure S6. Snapshots from simulations of varying Pe, $\phi$ with fixed $L = 21$, $f_\mathrm{a} = 0.5$. The frames at Pe $= 10$, $\phi = 0.4, 0.6, 0.8$ display nematic lanes did not reach a steady segregation state within our simulation time, and the frames shown are from the end of the trajectory.

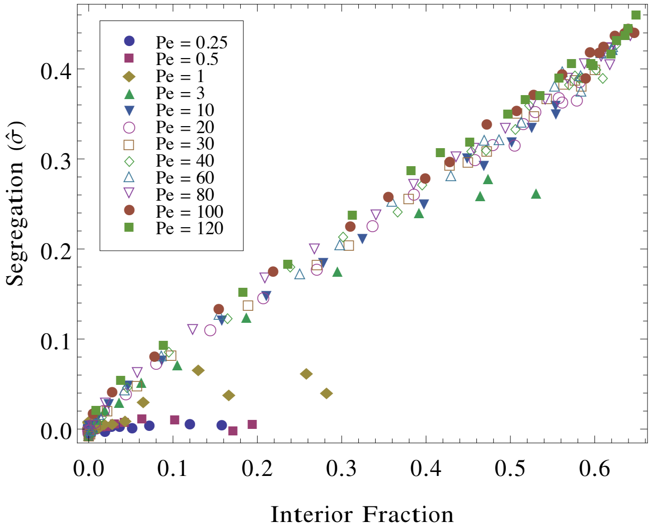


Figure S7. Comparison between the segregation parameter $\hat{\sigma}$ and the interior fraction $f_{\text{int}}$ for $L = 10$, $f_{\text{a}} = 0.5$ and $b = 5.0$. These parameters are highly correlated when clusters are sufficiently pure; the relationship does not hold for very low Pe, where the clusters identified are due only to number fluctuations.

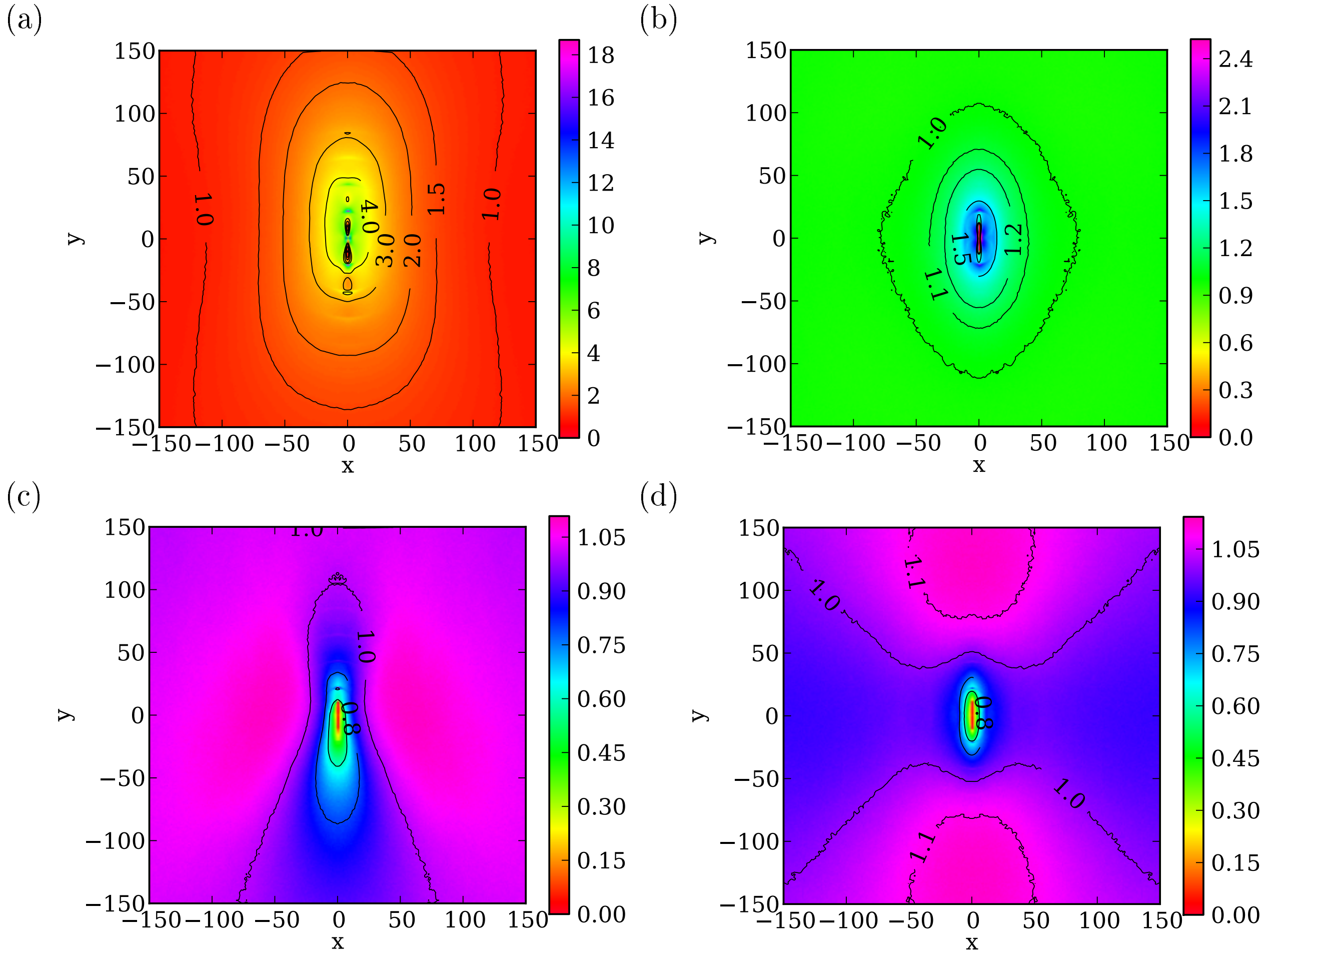


Figure S8. Pair correlation functions: (a) $G_{\mathrm{AA}}(x, y)$, (b) $G_{\mathrm{PP}}(x, y)$, (c) $G_{\mathrm{AP}}(x, y)$, (d) $G_{\mathrm{PA}}(x, y)$. Parameters are L=21, $\phi$=0.2, Pe=120.

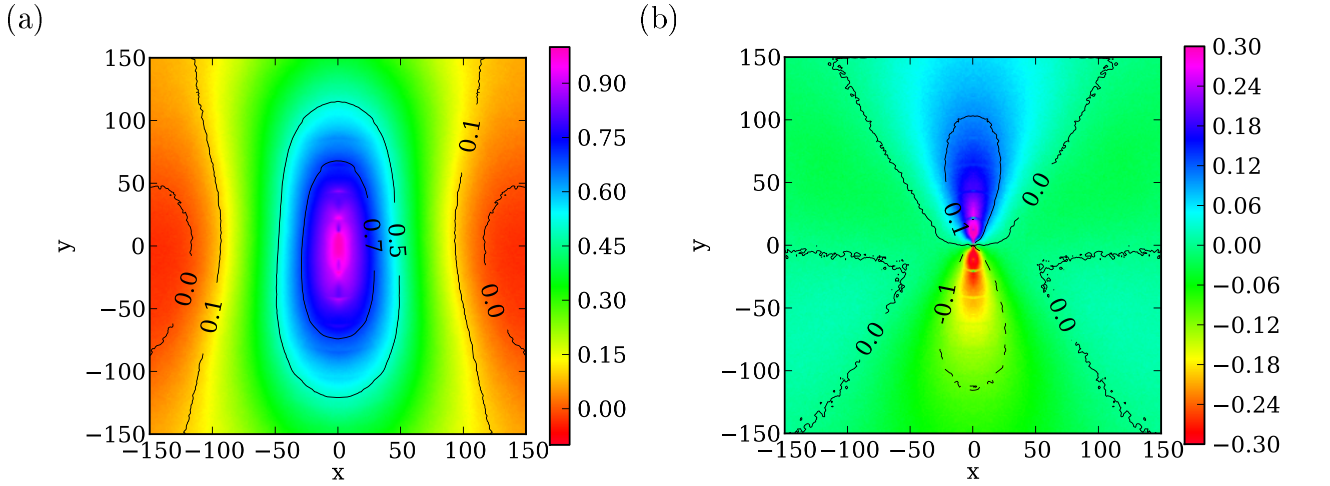


Figure S9. Polar orientation correlation functions: (a) $C_{\mathrm{P,AA}}(x, y)$, (a) $C_{\mathrm{P,PA}}(x, y)$. Parameters are L=21, $\phi$=0.2, Pe=120.

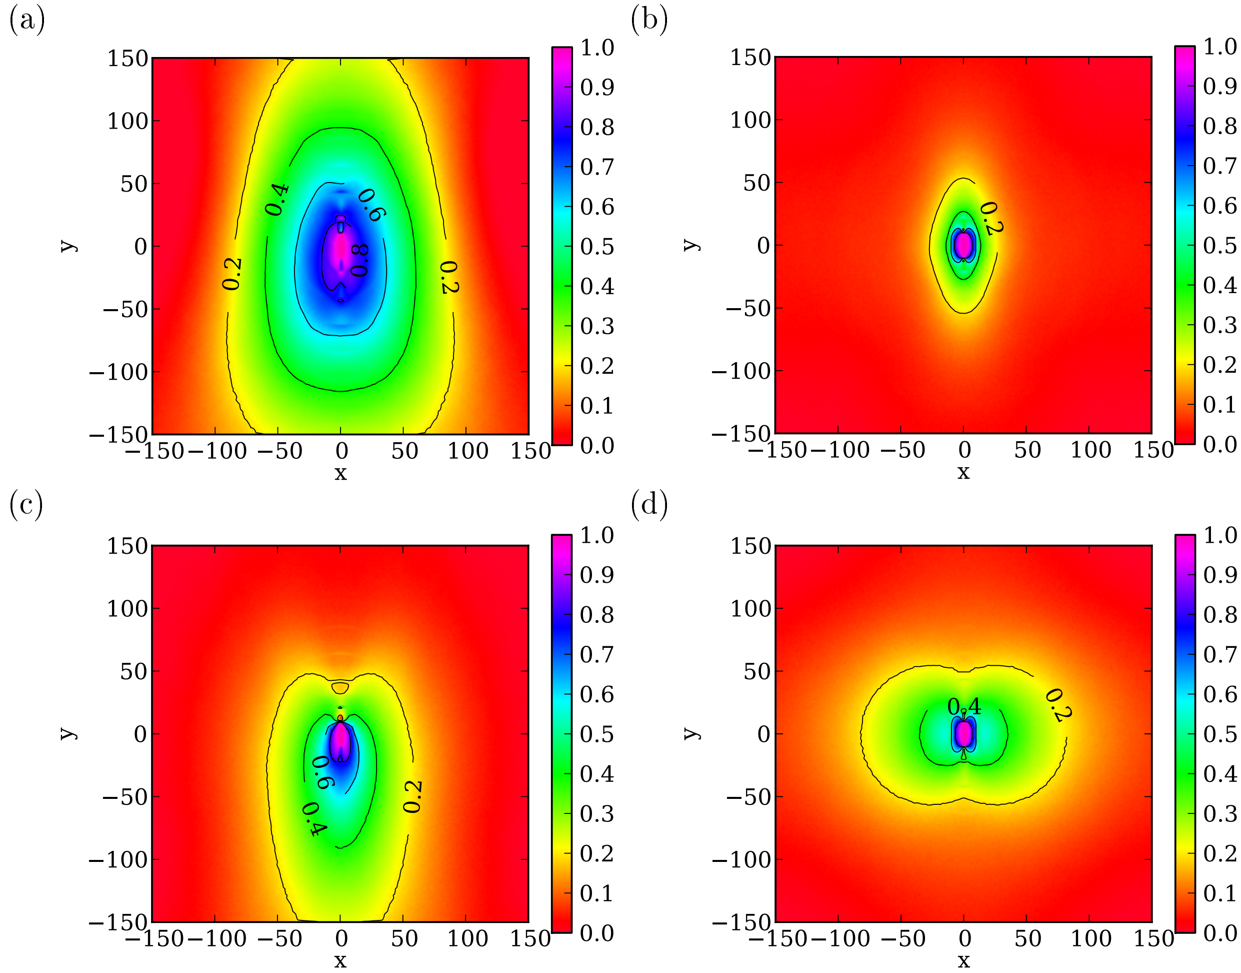


Figure S10. Nematic orientation correlation functions: (a) $C_{\mathrm{N,AA}}(x, y)$, (b) $C_{\mathrm{N,PP}}(x, y)$, (c) $C_{\mathrm{N,AP}}(x, y)$, (d) $C_{\mathrm{N,PA}}(x, y)$. Parameters are L=21, $\phi$=0.2, Pe=120.
